# Supplementary material for: SNAKE: Shape-aware Neural 3D Keypoint Field
Source: arXiv:2206.01724 source file (2022-10-17)
Supplement: Supplementary file 1 [file computation.tex]

\begin{tabular}{c|ccc|ccc}
    \toprule
    \multirow{2}[2]{*}{Input Point \#} & \multirow{2}[2]{*}{ISS} & \multirow{2}[2]{*}{USIP} & \multirow{2}[2]{*}{UKPGAN} & \multicolumn{3}{c}{Ours} \\
          &       &       &       & $J$=0 & $J$=5 & $J$=10 \\
    \midrule
    2048  & 0.07  &  0.006   & 14.41 & 0.08  & 0.50   & 0.81 \\
    4096  & 0.11  & 0.007  & 36.80 & 0.09  & 0.50   & 0.83 \\
    \bottomrule
\end{tabular}
